# Supplementary material for: Hand-waving and Interpretive Dance: An Introductory Course on Tensor Networks
Source: arXiv:1603.03039 ancillary file (2017-05-16)
Supplement: Supplementary file 1 [file TNSolutions.pdf]

# Hand-waving and Interpretive Dance: An Introduction to Tensor Networks **Solutions to Problems**

Jacob C. Bridgeman<sup>1</sup>, Christopher T. Chubb<sup>2</sup>

Centre for Engineered Quantum Systems  
School of Physics, The University of Sydney, Sydney, Australia

Version 4, May 16, 2017

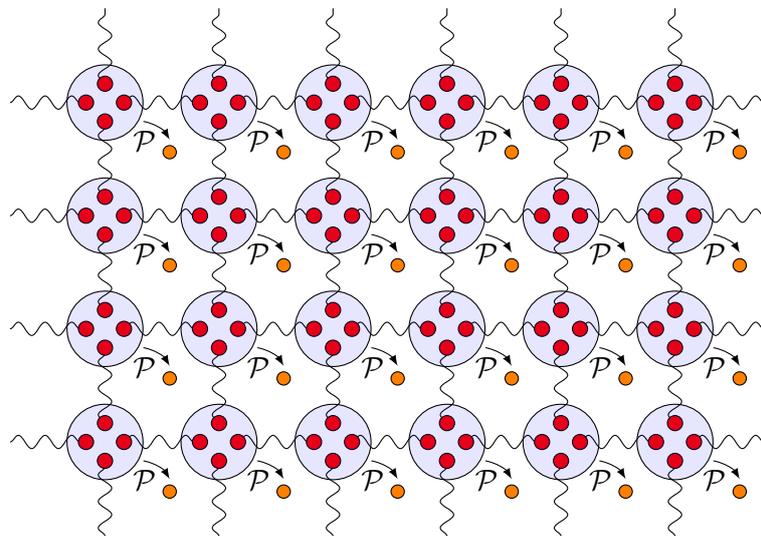

<sup>1</sup>[jacob.bridgeman@sydney.edu.au](mailto:jacob.bridgeman@sydney.edu.au), <http://www.physics.usyd.edu.au/~jbridge>  
<sup>2</sup>[christopher.chubb@sydney.edu.au](mailto:christopher.chubb@sydney.edu.au), <http://www.physics.usyd.edu.au/~chubb>

# Contents

|   |                                                |    |
|---|------------------------------------------------|----|
| 1 | Introduction to Tensor Networks                | 2  |
| 2 | Quantum information examples                   | 6  |
| 3 | Matrix Product States                          | 7  |
| 4 | Classifying Gapped Phases in 1D                | 10 |
| 5 | Tensor network algorithms                      | 12 |
| 6 | Projected Entangled Pair States                | 13 |
| 7 | Multiscale Entanglement Renormalisation Ansatz | 16 |

# 1 Introduction to Tensor Networks

## Solutions 1

1. Consider the following tensors, in which all indices are three-dimensional, indexed from 0:

$$\begin{array}{c} \textcircled{A} \\ | \\ j \end{array} \begin{array}{c} -i \\ \end{array} = i^2 - 2j, \quad \begin{array}{c} i \\ | \\ \textcircled{B} \\ | \\ k \end{array} \begin{array}{c} j \\ \end{array} = -3^i j + k, \quad (\text{Sols.1.1})$$

$$\begin{array}{c} j \\ | \\ \textcircled{C} \\ | \\ i \end{array} = j, \quad \begin{array}{c} i \\ | \\ \textcircled{D} \\ | \\ k \end{array} \begin{array}{c} j \\ \end{array} = ijk. \quad (\text{Sols.1.2})$$

Calculate the value of the following tensor network:

$$\begin{array}{c} \textcircled{A} \text{---} \textcircled{D} \\ | \quad | \\ \textcircled{B} \text{---} \textcircled{C} \end{array} \quad (\text{Sols.1.3})$$

First we begin by picking a global designation of the indices which is consistent with the contractions required:

$$\begin{array}{c} \textcircled{A} \\ | \\ \alpha \end{array} \begin{array}{c} -\beta \\ \end{array} = \beta^2 - 2\alpha, \quad \begin{array}{c} \alpha \\ | \\ \textcircled{B} \\ | \\ \delta \end{array} \begin{array}{c} \gamma \\ \end{array} = -3^\alpha \gamma + \delta, \quad (\text{Sols.1.4})$$

$$\begin{array}{c} \epsilon \\ | \\ \textcircled{C} \\ | \\ \delta \end{array} = \epsilon, \quad \begin{array}{c} \beta \\ | \\ \textcircled{D} \\ | \\ \epsilon \end{array} \begin{array}{c} \gamma \\ \end{array} = \beta\gamma\epsilon. \quad (\text{Sols.1.5})$$

Now that our indices have been matched up, the overall value of the tensor network  $T$  is given by the product of the above values, summed over all index labelling

$$T = \sum_{\alpha, \beta, \gamma, \delta, \epsilon=0}^2 A_{\alpha, \beta} B_{\alpha, \gamma, \delta} C_{\delta, \epsilon} D_{\beta, \gamma, \epsilon} \quad (\text{Sols.1.6})$$

$$= \sum_{\alpha, \beta, \gamma, \delta, \epsilon=0}^2 (\beta^2 - 2\alpha)(-3^\alpha \gamma + \delta)\beta\gamma\epsilon^2 \quad (\text{Sols.1.7})$$

$$= 1080. \quad (\text{Sols.1.8})$$

2. In this question we are going to consider expanding out a contraction sequence, in a manner which would be needed when coding up contractions. Given a network, and an associated bubbling, we wish to write out a table keeping track of the indices of the current object, the tensor currently being contracted in, the indices involved in that contraction, and new indices left uncontracted. For example for the network

$$\begin{array}{c} \textcircled{B} \\ / \quad \backslash \\ \alpha \quad \gamma \\ \textcircled{A} \quad \textcircled{C} \\ \backslash \quad / \\ \beta \quad \delta \end{array} \quad (\text{Sols.1.9})$$

where the bubbling is performed in alphabetical order, then the table in question looks like

| Current         | Tensor | Contract        | New             |
|-----------------|--------|-----------------|-----------------|
| –               | $A$    | –               | $\alpha, \beta$ |
| $\alpha, \beta$ | $B$    | $\alpha$        | $\gamma$        |
| $\beta, \gamma$ | $C$    | $\beta, \gamma$ | $\delta$        |

For the tensor network

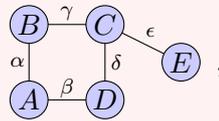

(Sols.1.10)

construct a corresponding table, where contraction is once again done in alphabetical order.

| Current                   | Tensor | Contract        | New                |
|---------------------------|--------|-----------------|--------------------|
| –                         | $A$    | –               | $\alpha, \beta$    |
| $\alpha, \beta$           | $B$    | $\alpha$        | $\gamma$           |
| $\beta, \gamma$           | $C$    | $\gamma$        | $\delta, \epsilon$ |
| $\beta, \delta, \epsilon$ | $D$    | $\beta, \delta$ |                    |
| $\epsilon$                | $E$    | $\epsilon$      | –                  |

3. (a) Calculate the contraction of the tensor network in Eq. (Notes.1.19) for bond dimension 3, i.e. calculate the number of three-colourings of the corresponding graph.

Numerically contracting the tensor network given in the notes gives a total number of vertex 3-colourings of 30.

- (b) Using the  $e$  and  $n$  tensors from Sec. Notes.1.5, come up with a construction for a tensor network which gives the number of *edge* colourings. For a planar graphs, construct an analogous network to count *face* colourings.

First we note that index values already correspond to edges, thus by simply placing an  $n$  tensor at every vertex of a graph, the tensor network given counts edge colourings.

As for a face colouring, we can simply apply the vertex colouring construction to the dual graph. As such we place  $e$  tensors on each face, and  $n$  on each edge, as below.

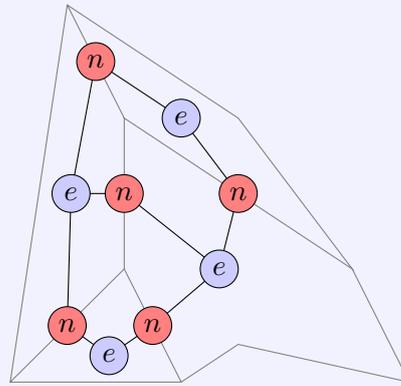

(Sols.1.11)

- (c) Using tensor networks, determine the minimum number of colours required to vertex and edge colour the below graph (known as the chromatic number and index respectively).

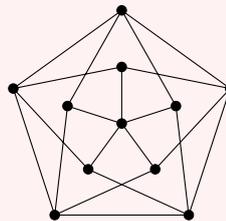

(Sols.1.12)

This is the Grötzsch Graph, it has chromatic number and index 4 and 5 respectively.

4. Much like the singular value decomposition, given a bisection of the indices we can consider norms of tensors.

- (a) Does the operator norm depend on the bisection, i.e. are the operator norms across any two bisections of the same tensor necessarily equal?

Yes it does depend on the bisection. A simple example is given by a generic matrix  $M$ . Treating it as a matrix, it has operator norm  $\|M\|_\infty$ . If however we vectorise  $M$ , treating it as a vector, then the operator norm of this vector corresponds to the Frobenius norm of the matrix  $\|M\|_F$ . In general these two norms differ, and thus the operator norm is bisection-dependent.

- (b) What about the Frobenius norm? If they can differ, give an example, if not draw a tensor network diagram that shows it to be manifestly independent of bisection.

For a matrix  $M$ , the square of the Frobenius norm is  $\text{Tr}(MM')$ . Taking a rank-3 tensor this looks like

$$\begin{array}{c} \text{---} \\ \text{---} \\ \text{---} \end{array} \left[ \bar{A} \right] \text{---} \left[ A \right] \begin{array}{c} \text{---} \\ \text{---} \\ \text{---} \end{array} . \quad (\text{Sols.1.13})$$

By simply wrapping the external leg around however we can see that this simply equals

$$\begin{array}{c} \text{---} \\ \text{---} \\ \text{---} \end{array} \left[ \bar{A} \right] \text{---} \left[ A \right] \begin{array}{c} \text{---} \\ \text{---} \\ \text{---} \end{array} . \quad (\text{Sols.1.14})$$

which is the squared Frobenius norm of the vectorisation. By a similar argument the Frobenius norm in any grouping can be shown to be equal to that of the vectorisation. Thus the Frobenius norm of a tensor is independent of the bisection with respect to which it is calculated.

$$\|A\|_F = \sqrt{\sum_{i_1, \dots, i_r} |A_{i_1, \dots, i_r}|^2}$$

5. Write out the Einstein notation corresponding to the network in Eq. (Notes.7.1).

The purpose of this exercise is to show that for networks for which the number of indices is too high for Einstein notation, TNN can remain legible.



### 3 Matrix Product States

#### Solutions 3

1. Describe the state given by an MPS with tensor

$$A = \begin{matrix} & 0 & 1 \\ 00 & \begin{pmatrix} 1 & 0 \\ 0 & 1 \end{pmatrix} \\ 10 & \\ 01 & \begin{pmatrix} 1/2 & -1/2 \\ 1/2 & -1/2 \end{pmatrix} \\ 11 & \end{matrix} \quad \begin{matrix} 1 - \boxed{A} - 3 \\ | \\ 2 \end{matrix}, \quad (\text{Sols.3.1})$$

where index ordering is as shown and indices 1 and 2 are combined. Boundary conditions require inserting a Pauli Z before closing periodic BCs, similar to Eq. (Notes.3.19).

Consider the self-inverse Hadamard gate. Performing a gauge transformation corresponding to contracting Hadamards onto each virtual bond, we end up with with a new MPS tensor

$$B = \begin{matrix} & 0 & 1 \\ 00 & \begin{pmatrix} 1 & 0 \\ 0 & 1 \end{pmatrix} \\ 10 & \\ 01 & \begin{pmatrix} 0 & 1 \\ 0 & 1 \end{pmatrix} \\ 11 & \begin{pmatrix} 0 & 0 \\ 0 & 0 \end{pmatrix} \end{matrix}. \quad (\text{Sols.3.2})$$

and a boundary condition now corresponding to closing on an  $X$  gate. We can recognise this as the MPS of Eq. (Notes.3.18), meaning that this described the W-state.

2. Describe the state given by the MPS whose only nonzero components are

$$0 - \boxed{A} - 0 \quad = \quad 1 - \boxed{A} - 1 \quad = \quad 0 - \boxed{A} - 1 \quad = \quad 1 - \boxed{A} - 0 \quad = 1, \quad (\text{Sols.3.3})$$

where the left and right boundary conditions are  $|0\rangle$ .

*Hint: Writing out the matrices corresponding to fixing the physical index might help!*

We have that

$$A_0 = \begin{pmatrix} 1 & 0 \\ 0 & 1 \end{pmatrix} = \mathbb{1}, \quad A_1 = \begin{pmatrix} 0 & 1 \\ 1 & 0 \end{pmatrix} = X. \quad (\text{Sols.3.4})$$

Therefore, if we begin on the left end in the  $\langle 0|$  state, we must insert an even number of  $A_1$  before we reach the right  $|0\rangle$ . Thus, we obtain the state

$$|\psi[A]\rangle = \sum |\text{even number of 1s}\rangle. \quad (\text{Sols.3.5})$$

3. Describe the qudit state given by the MPS

$$i - \begin{array}{c} \boxed{A} \\ | \\ j \end{array} - i \oplus j = 1 \quad (\text{Sols.3.6})$$

where  $i, j \in \mathbb{Z}_d$ ,  $\oplus$  denotes addition mod  $d$ , the left boundary condition is  $|0\rangle$ , and the right boundary is  $|q\rangle$  for some  $q \in \mathbb{Z}_d$ .

We have that

$$A_1 = \begin{pmatrix} 0 & 1 & 0 & \cdots & 0 & 0 & 0 \\ 0 & 0 & 1 & \cdots & 0 & 0 & 0 \\ 0 & 0 & 0 & \cdots & 0 & 0 & 0 \\ \vdots & \vdots & \vdots & \ddots & \vdots & \vdots & \vdots \\ 0 & 0 & 0 & \cdots & 0 & 1 & 0 \\ 0 & 0 & 0 & \cdots & 0 & 0 & 1 \\ 1 & 0 & 0 & \cdots & 0 & 0 & 0 \end{pmatrix} \quad (\text{Sols.3.7})$$

We can recognise  $A_1$  as the (transpose of) the generalised Pauli  $X$  matrix and  $A_k = A_1^k$ . Therefore, if we begin on the left end in the  $\langle 0|$  state, we must insert  $A_k$ s such that the sum of the string (mod  $d$ ) is  $q$  before we reach the right  $|q\rangle$ . Thus, we obtain the state

$$|\psi[A]\rangle = \sum |\text{strings summing to } q\rangle. \quad (\text{Sols.3.8})$$

4. Let  $\mathcal{G}$  be some group. Describe the operator given by the MPO with

$$g - \begin{array}{c} h \\ | \\ \boxed{M} \\ | \\ h \end{array} - g \cdot h = 1 \quad (\text{Sols.3.9})$$

where the left boundary condition is  $0$ , the right boundary is some group element  $q$  and  $\cdot$  denotes group multiplication.

This is a generalisation of problem 3. Rather than a state, we end up with an operator. Rather than summing to  $q$ , the operator terms should multiply to  $q$  (under the group operation). We end up with the operator which projects onto states which multiply to  $q$ .

5. Suppose the local basis is labelled by particle number. What is the action of the following operator (bond dimension linearly increasing left to right)?

$$n - \begin{array}{c} m \\ | \\ \boxed{M} \\ | \\ m \end{array} - n + m = 1 \quad (\text{Sols.3.10})$$

with left vector  $L = |0\rangle$  and right vector  $R = \sum_{i=0}^N i|i\rangle$ .

This is similar to the operator in problem 4, however rather than projecting onto a subspace, the operator multiplies a state summing to  $j$  by the number  $j$ . Therefore, taking expectations of this operator returns the expected particle number.

6. Write an MPO for the transverse-field-cluster Hamiltonian

$$H = -J \sum_j Z_{j-1} X_j Z_{j+1} - h \sum_j X_j. \quad (\text{Sols.3.11})$$

*Hint: This can be done with bond dimension 4.*

We can use the construction in Appendix Notes.A, we obtain

$$M = \begin{pmatrix} \mathbb{1} & 0 & 0 & 0 \\ Z & 0 & 0 & 0 \\ 0 & X & 0 & 0 \\ -hX & 0 & -JZ & \mathbb{1} \end{pmatrix}, \quad (\text{Sols.3.12})$$

with left and right vectors

$$L = (0 \ 0 \ 0 \ 1) \quad R = (1 \ 0 \ 0 \ 0)^T. \quad (\text{Sols.3.13})$$

7. Use the ideas of MPSs and MPOs to prove that log depth quantum circuits can be simulated efficiently on a classical computer.

Suppose we have a log depth circuit acting on  $|0\rangle^{\otimes N}$ . Breaking  $U$  down in to circuit elements, the state we wish to know has the form

$$\psi \xrightarrow{U} = \text{circuit} \xrightarrow{\log(n)} \text{product of states} \quad (\text{Sols.3.14})$$

Next we decompose our gates into single qubit tensors:

$$\text{blue box} = \text{blue box} \text{ with red box} = \text{red box} \text{ followed by green box} \quad (\text{Sols.3.15})$$

We now use this factorisation, and vertically group our tensors together. The resulting state is an MPS.

$$\text{circuit} = \text{chain of pink boxes} \quad (\text{Sols.3.16})$$

As our circuit has only logarithmic depth, the bond dimension is at most polynomial, allowing our classical simulation to be efficient.

## 4 Classifying Gapped Phases in 1D

### Solutions 4

1. The group  $\mathbb{Z}_2 \times \mathbb{Z}_2$  has the presentation  $\mathbb{Z}_2 \times \mathbb{Z}_2 = \langle x, z | x^2 = z^2 = e, xz = zx \rangle$ . Show that the Pauli matrices form a projective representation of  $\mathbb{Z}_2 \times \mathbb{Z}_2$ .

*Hint: let  $v_x = X$ ,  $v_z = Z$ ,  $v_{xz=zx} = Y$  and show that  $v_g v_h = \omega[g, h] v_{gh}$ , where  $\omega$  is some phase.*

Let  $v_x = X$ ,  $v_z = Z$  and  $v_{xz} = Y$ . We can then calculate  $\omega[g, h]$ , obtaining

$$\begin{array}{c} e \quad x \quad z \quad xz \\ e \quad \begin{pmatrix} 1 & 1 & 1 & 1 \\ 1 & 1 & -i & i \\ 1 & i & 1 & -i \\ 1 & -i & i & 1 \end{pmatrix} \end{array} \quad (\text{Sols.4.1})$$

2. Determine the factor system  $\omega[g, h]$  for the Pauli matrices.

See Problem 1 above.

3. Show that the Pauli projective representation is not equivalent to a linear representation.

*Hint:  $xz = zx$ , can we rephase  $v_x$  and  $v_z$  to make  $v_x v_z - v_z v_x = 0$ ?*

If we had a linear representation, we would have  $u_x u_z - u_z u_x = 0$ . Consider rephasing the  $v$ s

$$v_g \rightarrow e^{i\phi_g} v_g. \quad (\text{Sols.4.2})$$

The commutator then becomes

$$e^{i(\phi_x + \phi_z)} (v_x v_z - v_z v_x). \quad (\text{Sols.4.3})$$

Therefore no rephasing can bring this to 0, so the Paulis do *not* form a linear representation.

4. Recall from Section Notes.3.2 that the symmetry of the cluster state is  $\mathbb{Z}_2 \times \mathbb{Z}_2$ , with the action on the MPS tensor being

$$\begin{array}{c} \text{[Diagram 1]} \\ \text{[Diagram 2]} \end{array} = \begin{array}{c} \text{[Diagram 3]} \\ \text{[Diagram 4]} \end{array} \quad (\text{Sols.4.4})$$

What can we conclude about the cluster state?

Since the Paulis form a nontrivial projective representation of  $\mathbb{Z}_2 \times \mathbb{Z}_2$ , we know that the cluster state is in a nontrivial phase. That is, it cannot be transformed into a product state using a constant depth local circuit with  $\mathbb{Z}_2 \times \mathbb{Z}_2$  symmetry.

## 5 Tensor network algorithms

### Solutions 5

1. Consider the critical transverse Ising model

$$H = - \sum_{i=1}^{n-1} X_i X_{i+1} - \sum_{i=1}^n Z_i. \quad (\text{Sols.5.1})$$

For open boundary conditions, it is known that the ground state energy as a function of  $n$  has the form

$$E(n) = 1 - \csc\left(\frac{\pi}{\alpha n + \beta}\right) \quad (\text{Sols.5.2})$$

for some integers  $\alpha$  and  $\beta$ . Using either DMRG or TEBD, estimate the ground state energy for several chain lengths and calculate  $\alpha$  and  $\beta$ .

Running this for moderate system sizes, bond dimensions, and time-scales, with either DMRG or TEBD, it is relatively easy to calculate that  $\alpha = 4$ ,  $\beta = 2$ .

2. It is known that the LOCAL HAMILTONIAN problem is in  $\mathbf{P}$  for gapped Hamiltonians. DMRG and TEBD are the most common techniques for numerically finding the ground states of such systems. For a gapped and 1D local Hamiltonian, prove that DMRG or TEBD converge.

This was a somewhat of trick question. Despite the complexity of the underlying problem and the practical power of these algorithms both being well understood, a satisfactory theoretical understanding of the effectiveness of DMRG/TEBD is an elusive open problem. Even a concrete statement of the convergence properties that these algorithms possess is still a topic of debate.

## 6 Projected Entangled Pair States

### Solutions 6

1. What is the PEPS tensor required to build the GHZ state on the honeycomb lattice where spins reside on vertices?

Let the PEPS tensor be the ‘delta-tensor’, the tensor which is 1 if all indices are equal and zero otherwise. Fixing boundary conditions to be  $|+\rangle$  on each index give the GHZ state.

2. Which 2 qubit gate is obtained by contracting the following tensors along the horizontal index?

$$\begin{array}{c} j \\ | \\ \boxed{u} \\ | \\ i \end{array} - k = \delta_{i,j} (\delta_{k,0} + (-1)^i \delta_{k,1}), \quad \begin{array}{c} y \\ | \\ \boxed{v} \\ | \\ x \end{array} = \delta_{x,y,z}. \quad (\text{Sols.6.1})$$

Performing the contraction over the horizontal bond, we obtain

$$\begin{array}{cc} & \begin{array}{cccc} 00 & 10 & 01 & 11 \end{array} \\ \begin{array}{c} 00 \\ 10 \\ 01 \\ 11 \end{array} & \left( \begin{array}{cccc} 1 & 0 & 0 & 0 \\ 0 & 1 & 0 & 0 \\ 0 & 0 & 1 & 0 \\ 0 & 0 & 0 & -1 \end{array} \right), \quad (\text{Sols.6.2})
 \end{array}$$

where the row indices are  $(ix)$  and the column indices are  $(jy)$ . We recognise this as the  $CZ$  gate.

3. The cluster state can be prepared from the all  $|+\rangle$  state by applying  $CZ$  between all adjacent spins. Show that Eq. (Notes.6.20) indeed gives the cluster state.

*Hint: Consider the decomposition of a gate given in the above problem.*

We have a decomposition of the  $CZ$  operator in 2. It remains to build a PEPS tensor from this. The only tricky part is ensuring that when the bonds link up, each ‘ $u$ ’ tensor connects to a ‘ $v$ ’ tensor. The PEPS tensor is therefore

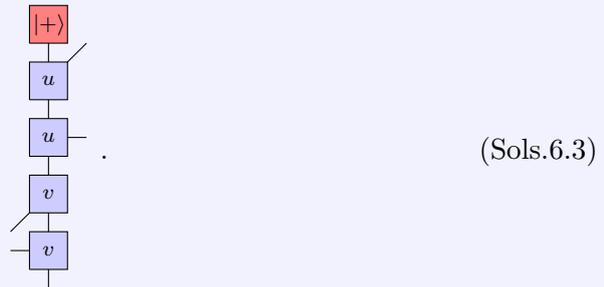

Contracting this, we obtain the tensor in Eq. (Notes.6.20).

- Investigate how logical operators on the physical spins of the Toric code can be pulled onto the virtual level of the PEPS. Can you see why  $\mathcal{G}$ -injectivity is so important for topologically ordered PEPS?

The logical operators of the Toric code are build from strings of  $Z$ s and  $X$ s. Consider placing a single  $Z$  on a physical bond of the PEPS tensor in Eq. (Notes.6.17). It is not hard to see that

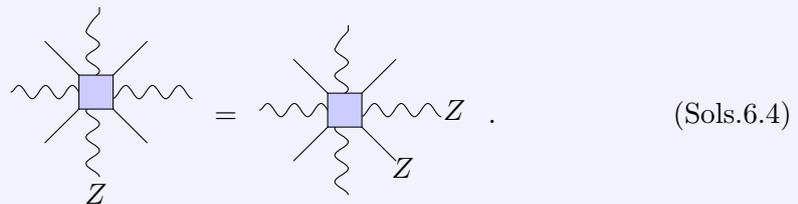

We can use this to understand how the physical  $Z$  string pulls through to the virtual level.

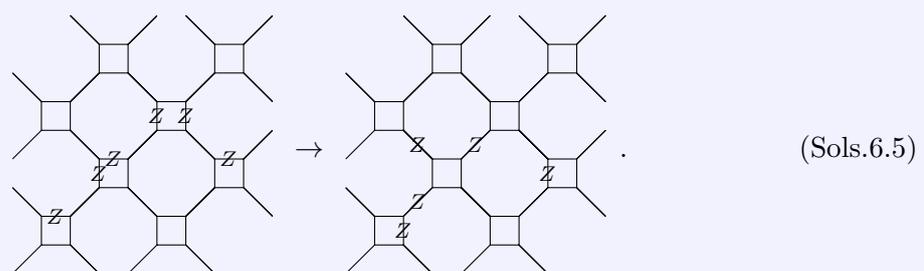

Which has two physical  $Z$ s corresponding to the end points of the string, and a virtual string of  $Z$ s. This string can be moved around using the rules of Eq. (Notes.6.19).

We can do the same exercise for the  $X$  string and obtain

(Sols.6.6)

(Sols.6.7)

Thus, the  $X$  string pulls through to an isolated pair of  $X$ s acting on the virtual level at the ends of the string.

The  $\mathcal{G}$ -injectivity property is the ability to pull the  $Z$  string through the PEPS tensor, which means the presence of a  $Z$  string is not locally observable.

5. Convince yourself that evaluating expectation values on the PEPS constructed from a classical partition function indeed reproduces the thermal expectation values.

Play with the network! Pull the expectation up to the virtual level and flatten.

## 7 Multiscale Entanglement Renormalisation Ansatz

### Solutions 7

1. Can you find a MERA for the W state?

For this we are going to construct a tree ( $u = \mathbb{1}$ ) that takes the W-state  $n$  qubits to the W-state on  $2n$  qubits.

$$\begin{array}{c} 0 \\ \triangle \\ 0 \quad 0 \end{array} = \begin{array}{c} 1 \\ \triangle \\ 1 \quad 0 \end{array} = \begin{array}{c} 1 \\ \triangle \\ 0 \quad 1 \end{array} = 1 \quad (\text{Sols.7.1})$$

It can be seen that by applying this isometry to a W-state will expand it. Thus if we take a tree with top tensor  $T = |1\rangle$ , then we recover the full W-state.

2. What state is given by the MERA with

$$\begin{array}{c} \triangle \\ \parallel \\ \parallel \end{array} = \begin{array}{c} \text{ } \\ \text{ } \\ \text{ } \end{array}, \quad (\text{Sols.7.2})$$

$u = \mathbb{1}$  and top tensor  $T = \frac{1}{\sqrt{2}}(|00\rangle + |11\rangle)$ ?

Firstly note that the top tensor  $T \propto |00\rangle + |11\rangle$  is simply the Bell state, i.e.  $T = \bigwedge$ . Drawing the tree out for 8 sites (16 qubits), we have:

$$\text{Tree structure} = \text{Layer of 8 Bell states} \quad (\text{Sols.7.3})$$

We therefore have the periodic state consisting of Bell states shared between each neighbouring site, i.e. the state on which PEPS is based. As a result we can see that any MPS state can therefore be prepared from a MERA by modifying one single layer.

3. The above state is the ground state of the Hamiltonian

$$H = - \sum_{j=1}^{N/2} (X_{2j} X_{2j+1} + Z_{2j} Z_{2j+1}) \quad (\text{Sols.7.4})$$

on periodic boundary conditions. Is that clear? Can you find a unitary  $U_{2j-1,2j}$  which transforms this Hamiltonian into

$$H = - \sum_{j=1}^{N/2} (Z_{2j-1} X_{2j} Z_{2j+1} + Z_{2j} X_{2j+1} Z_{2j+2})? \quad (\text{Sols.7.5})$$

Let  $U_{2j-1,2j} = (\mathbb{1} \otimes h)CZ$ , where  $h$  is the Hadamard gate, and let  $U = \bigotimes_j U_{2j-1,2j}$ , then  $U^\dagger H U$  is as desired.

4. Act with the above transformation  $U$  on the MERA tensor to obtain another MERA tensor. What is this state?

We want this to be a ground state of the transformed Hamiltonian, so we need  $U^\dagger |\psi\rangle$ . If we transform the lower indices on the second layer of the MERA with  $U^\dagger$  (so that each tensor is identical), then we must transform the upper indices of the lower layer (i.e. ensure that above the physical layer,  $U$  is acting as a gauge transformation). The tensor we obtain is

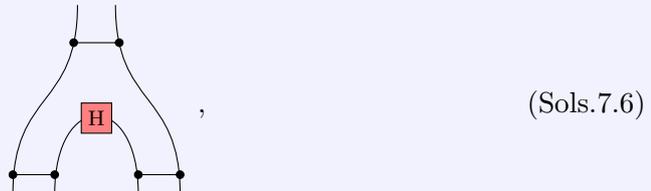

so this is the cluster state.

5. What is the maximum range of thermodynamic observables in a ternary MERA scheme?

We can easily see this by examining the causal cones (indicated by a line) of various sized operators in the MERA. We see that there is one special location where 3 site operators are maintained (red line). Elsewhere, each operator eventually shrinks to two sites (blue lines).

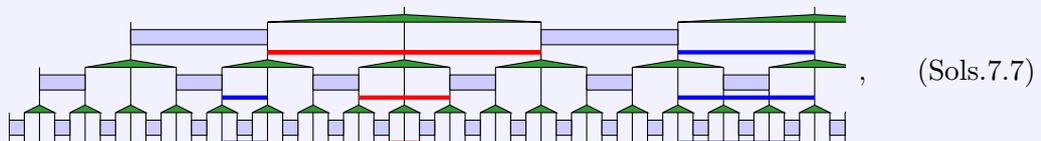

6. What does the reduced density matrix on a few sites of the MERA look like? Notice that it corresponds to the top tensor being passed through a CPTP map several times, this is usually called the *descending superoperator*.

Consider taking the MERA in Eq. (Notes.7.11), and look at the reduced density matrix on the support of the operator.

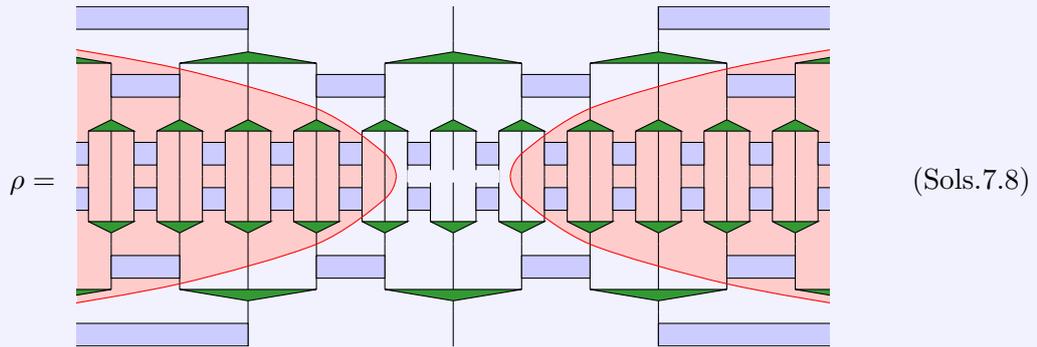

Note that in the above diagram, the five pairs of leg near the centre of the diagram are unconnected, corresponding to the reduced density matrix – all other physical legs are connected corresponding to the partial trace. Firstly we notice that everything outside of the light code (red shaded region) cancels out. Using this, and flipping the diagram inside out, we get that the reduce density matrix has the form:

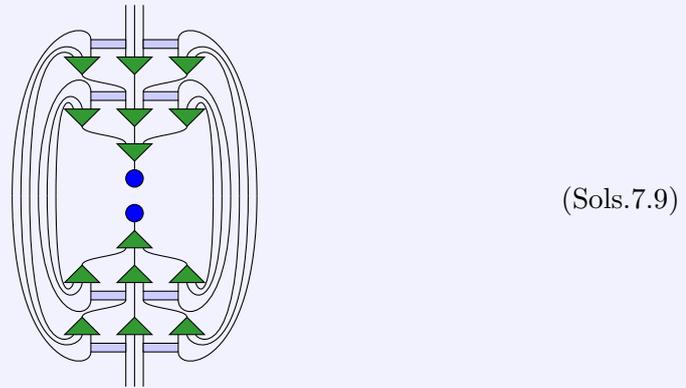

where the blue circle is the top tensor  $T$ . We can see that this simply corresponds to applying the map dual to the descending super-channel multiple times

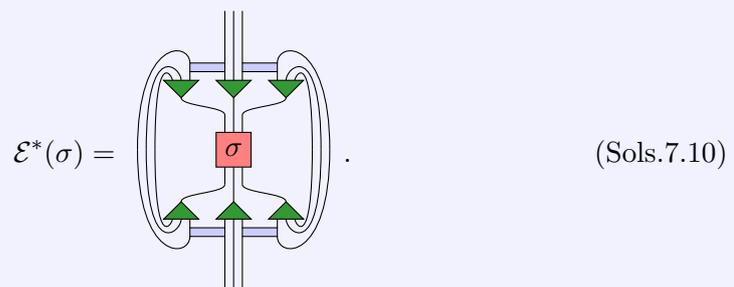

Thus we see that reduced density matrices generally take the form

$$\rho = (\mathcal{E}^*)^n (|T\rangle\langle T|). \tag{Sols.7.11}$$

7. Do tree tensor networks (i.e. MERA for  $u = 1$ ) have any area law violation on contiguous regions?

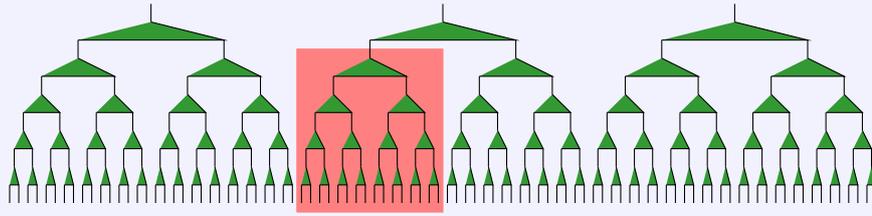

(Sols.7.12)

The indicated region (and any similar subtree) can be removed by cutting a single bond. Therefore, the area law is not violated on such regions.
